# Supplementary material for: On Neural Network Equivalence Checking using SMT Solvers
Source: arXiv:2203.11629 source file (2022-03-22)
Supplement: Supplementary file 1 [file appendix.tex]

\pagebreak
\section{Case Study: Neural Network Controller \& Approximate Equivalence}
This case study is proposed by Chih-Hong and can be used (i) as a part of the AUTh work within FOCETA, and (ii) as a benchmark for approximate equivalence checking of neural networks; when employed as controllers.

\paragraph{Short Description for Haris}~\\
The data are saved as MATLAB arrays (.mat) and are generated from a script provided from Mathworks\footnote{https://www.mathworks.com/help/reinforcement-learning/ug/imitate-mpc-controller-for-lane-keeping-assist.html}. The autogenerated data array contains 9 variables but we only keep 7 (inputs+targets). I wrote a small script to convert the data to numpy arrays or load them in Python. Note that the first 6 columns contain the inputs and the last row the output/target. We have 100,000 samples; can be seen as instances. The rows represent the inputs and columns the instances/samples. The numpy object is stored as {\tt nikos\_mpc.pkl}. A text file {\tt nikos\_mpc.txt}is also provided. 
To load the pickled file into Python (tested with Python 3), run 
\begin{center}
\begin{BVerbatim}
    import pickle
    import numpy as np
    with open('nikos_mpc.pkl', 'rb') as fin : 
    data = pickle.load(fin)
\end{BVerbatim} 
\end{center}

\noindent To load the TXT file, you can use
\begin{center}
\begin{BVerbatim}
data = np.genfromtxt('nikos_mpc.txt', delimiter=',')
X=data(:-1,:)
y=data(-1,:)
\end{BVerbatim} 
\end{center}
The structure of the NN is given in Table~\ref{tab:structure}.
The training parameters are given in Table~\ref{tab:training_param}.
\begin{table*}[ht!]\centering
\caption{Neural Network Training -- Parameters }\vspace{0.2em}
\begin{tabular}{@{}lcl@{}}
\toprule
\textbf{Type/Parameter} & \textbf{Answer/Value} & \textbf{Remarks}\\
\midrule
    training algorithm & adam & \\
    \# epochs & 30&\\
    minibatch size & 512&\\
    \% of test data & 5\%\\
    \% of validation data & 10\%\\
     \bottomrule
\end{tabular}
\label{tab:training_param}
\end{table*}%

\clearpage
\begin{table*}[ht!]\centering
\caption{Neural Network structure }\vspace{0.2em}
\begin{tabular}{@{}lcl@{}}
\toprule
\textbf{Type/Parameter} & \textbf{Answer/Value} & \textbf{Remarks}\\
\midrule
    NN type & feedforward & \\
    problem & regression& \\
     \# hidden layers & 3&\\
     \#neurons per layer & 45, 45, 45 &\\
     activ. function & ReLU, ReLU, ReLU &\\
     input layer & 1 &\\
     \# inputs & 6 & time-series data\\
     output layer & 1&\\
     activ. function of output & Tanh&\\
     scaling of output & 1.04 & scaling layer\\
     \# outputs & 1& time-series\\
     \bottomrule
\end{tabular}
\label{tab:structure}
\end{table*}%

\begin{table*}[ht!]\centering
\caption{Model Parameters -- Constraints }\vspace{0.2em}
\begin{tabular}{@{}lcl@{}}
\toprule
\textbf{Type/Parameter} & \textbf{Answer/Value} & \textbf{Remarks}\\
\midrule
    output/target & $[-1.04, 1.04]$ & steering angle $[-60,60]$ \\
    sampling time & 0.1&\\
    input range $x_1$ & [-2,2] & $v_x$ (m/s) \\
    input range $x_2$ & [-1.04, 1.04]& rad/s\\
    input range $x_3$ & [-1,1] &m \\
    input range $x_4$ & [-0.8, 0.8]& rad\\
    input range $x_5$ & [-1.04, 1.04] & $u_0$ (steering angle)\\
    input range $x_6$ & [-0.01,0.01] & $\rho$\\
     \bottomrule
\end{tabular}
\label{tab:training_param}
\end{table*}%
As mentioned in one of the emails, the next tasks (of Haris) involve:

\begin{enumerate}
    \item Write a script to create a Neural Network in Python, replicating the exact structure.
    \item Design two NNs, e.g. change the number of epochs.
    \item Choose an $\epsilon$ bound and perform approximate equivalence checking.
\end{enumerate}
